# Supplementary material for: Sharpness-Aware Minimization Improves Language Model Generalization
Source: arXiv:2110.08529 source file (2022-03-15)
Supplement: Supplementary file 1 [file appendix.tex]

% ==================

\section*{Full zero-shot multilingual experimental results}
\begin{table*}[!t]
\tiny
    \centering
    \begin{tabular}{l|c|ccccccccc}
    \toprule
        Model &	avg & en & ar & bn & fi & id & ko & ru & sw & te \\
    \midrule
Small & 31.2 / 20.9 & 54.2 / 42.7 & 34.8 / 21.1 & 19.6 / 14.2 & 30.0 / 18.2 & 37.0 / 25.5 & 25.7 / 19.2 & 33.3 / 19.1 & 31.3 / 19.4 & 14.7 / 8.5 \\
Small + SAM (0.05) & 30.8 / 18.8 & 57.0 / 44.5 & 38.4 / 21.8 & 12.3 / 7.1 & 29.4 / 15.2 & 36.8 / 21.4 & 24.1 / 16.3 & 32.4 / 16.1 & 32.9 / 17.4 & 13.9 / 9.6 \\
\midrule
Base & 44.2 / 30.9 & 65.9 / 53.0 & 51.2 / 32.8 & 30.6 / 17.7 & 47.3 / 32.7 & 50.2 / 35.0 & 34.7 / 26.4 & 42.9 / 24.3 & 42.5 / 29.9 & 32.3 / 25.9 \\
Base + SAM (0.15) & 50.1 / 34.8 & 70.1 / 58.6 & 58.0 / 36.7 & 33.8 / 21.2 & 55.8 / 40.5 & 61.8 / 42.3 & 42.4 / 32.2 & 45.7 / 22.4 & 53.0 / 35.5 & 30.5 / 24.1 \\
\midrule
Large & 63.7 / 44.6 & 76.3 / 64.1 & 65.0 / 42.3 & 56.4 / 35.4 & 68.7 / 51.3 & 70.3 / 49.6 & 59.7 / 48.2 & 56.0 / 30.3 & 64.5 / 43.1 & 56.3 / 36.8 \\
Large + SAM (0.15) & 49.9 / 30.9 & 72.9 / 56.4 & 47.2 / 24.0 & 23.4 / 14.2 & 56.8 / 34.7 & 59.4 / 33.1 & 45.3 / 32.6 & 37.5 / 16.4 & 60.5 / 37.9 & 46.3 / 28.8 \\
        \bottomrule
    \end{tabular}
    \caption{Results for zero-shot TyDiQA-GoldP.}
    \label{tab:zeroshot_tydiqa_full}
\end{table*}

\begin{table*}[!t]
\small
    \centering
    \begin{tabular}{l|c|ccccccccc}
    \toprule
        Model (95\%) &	SGlue &	BoolQ &	CB & 	CoPA & MultiRC &	ReCoRD &	RTE & 	WiC &	WSC \\ 
        \midrule
Small & 55.7 & 63.0 & 47.4 / 67.9 & 58.0 & 63.4 / 16.5 & 47.4 / 46.0 & 60.3 & 58.6 & 61.5 \\
Small + SAM (0.05) & 56.2 & 63.1 & 49.9 / 71.4 & 56.0 & 63.9 / 17.2 & 48.4 / 47.0 & 56.7 & 60.3 & 64.4 \\
\midrule
Base & 62.0 & 65.8 & 48.7 / 69.6 & 62.0 & 67.7 / 21.5 & 64.4 / 62.8 & 68.2 & 62.4 & 70.2 \\
Base + SAM (0.15) & 64.7 & 71.5 & 50.5 / 71.4 & 68.0 & 72.1 / 27.8 & 66.0 / 64.1 & 68.6 & 62.4 & 71.2 \\
\midrule
Large & 75.1 & 83.1 & 72.0 / 87.5 & 78.0 & 78.6 / 40.4 & 80.8 / 78.8 & 80.5 & 69.0 & 71.2 \\
Large + SAM (0.15) & 75.6 & 82.8 & 60.2 / 85.7 & 78.0 & 79.2 / 43.0 & 80.8 / 79.1 & 80.5 & 70.4 & 78.8 \\
\midrule
XL & x & x & x & x & x & x & x & x & x \\ 
XL + SAM & x & x & x & x & x & x & x & x & x \\ 
        \bottomrule
    \end{tabular}
    \caption{20\% data, 95-percentile.}
    \label{tab:finetune_superglue_20_95}
\end{table*}

\begin{table*}[t]
    \centering
    \begin{tabular}{l|c|ccccccccc}
    \toprule
        Model &	Glue &	CoLA& SST& MRPC	& STSB & QQP & MNLI& QNLI& RTE \\ 
        \midrule
T5.1.1 Small & x & x & x & x & x & x & x & x & x \\ 
T5.1.1 Small + SAM & x & x & x & x & x & x & x & x & x \\
\midrule
T5.1.1 Base & x & x & x & x & x & x & x & x & x \\ 
T5.1.1 Base + SAM & x & x & x & x & x & x & x & x & x \\
\midrule
T5.1.1 Large & x & x & x & x & x & x & x & x & x \\ 
T5.1.1 Large + SAM & x & x & x & x & x & x & x & x & x \\
\midrule
T5.1.1 XL & x & x & x & x & x & x & x & x & x \\ 
T5.1.1 XL + SAM & x & x & x & x & x & x & x & x & x \\ 
\bottomrule
    \end{tabular}
    \caption{Experimental results (dev scores) on the GLUE benchmark.Models  are pre-trained with and without SAM on the C4 corpus for $500k$ and subsequently fine-tuned without SAM for $250k$ steps. Results are averaged over four runs, and entries that are within two standard errors of the optimal are bolded. We see that SAM improves performance across \emph{all} model sizes.}
    \label{tab:pretrain_glue}
\end{table*}

\begin{table*}[t]
\small
    \centering
    \begin{tabular}{l|c|ccccccccc}
    \toprule
        Model (95\%) &	SGlue &	BoolQ &	CB & 	CoPA & MultiRC &	ReCoRD &	RTE & 	WiC &	WSC \\ 
        \midrule
Small & 65.6 & 71.9 & 85.3 / 85.7 & 64.0 & 67.1 / 20.7 & 59.3 / 58.0 & 67.1 & 63.2 & 70.2 \\
Small + SAM (0.05) & 65.7 & 73.1 & 84.1 / 85.7 & 56.0 & 67.1 / 21.6 & 59.0 / 57.9 & 68.6 & 63.8 & 76.0 \\
\midrule
Base & 73.4 & 79.6 & 86.5 / 91.1 & 69.0 & 75.0 / 34.2 & 74.0 / 72.7 & 79.8 & 68.2 & 74.0 \\
Base + SAM (0.15) & 75.2 & 81.6 & 87.4 / 91.1 & 72.0 & 76.3 / 37.0 & 75.3 / 74.0 & 83.8 & 69.0 & 75.0 \\
\midrule
Large & 82.0 & 86.1 & 96.7 / 96.4 & 83.0 & 82.5 / 49.1 & 84.5 / 83.5 & 87.0 & 71.9 & 81.7 \\
Large + SAM (0.15) & 83.1 & 87.3 & 93.6 / 96.4 & 82.0 & 83.4 / 51.5 & 86.3 / 85.2 & 88.4 & 73.5 & 85.6 \\
\midrule
XL & 84.5 & 88.2 & 90.4 / 92.9 & 89.0 & 85.9 / 57.8 & 88.0 / 86.8 & 90.3 & 73.8 & 83.7 \\
XL + SAM (0.15) & 87.6 & 89.1 & 96.2 / 98.2 & 94.0 & 87.2 / 61.0 & 90.2 / 89.2 & 91.0 & 74.9 & 90.4 \\
        \bottomrule
    \end{tabular}
    \caption{superglue 100\%, 95-percentile.}
    \label{tab:finetune_superglue_95}
\end{table*}

\begin{table*}[t]
    \centering
    \begin{tabular}{l|c|ccccccccc}
    \toprule
        Model &	Glue &	CoLA& SST& MRPC	& STSB & QQP & MNLI& QNLI& RTE \\ 
        \midrule
T5.1.1 Small & x & x & x & x & x & x & x & x & x \\ 
T5.1.1 Small + SAM & x & x & x & x & x & x & x & x & x \\
\midrule
T5.1.1 Base & x & x & x & x & x & x & x & x & x \\ 
T5.1.1 Base + SAM & x & x & x & x & x & x & x & x & x \\
\midrule
T5.1.1 Large & x & x & x & x & x & x & x & x & x \\ 
T5.1.1 Large + SAM & x & x & x & x & x & x & x & x & x \\
\midrule
T5.1.1 XL & x & x & x & x & x & x & x & x & x \\ 
T5.1.1 XL + SAM & x & x & x & x & x & x & x & x & x \\ 
\bottomrule
    \end{tabular}
    \caption{Experimental results (dev scores) on the GLUE benchmark. Public checkpoints of various sizes are fine-tuned with and without SAM for 250k steps. Results are averaged over four runs, and entries that are within two standard errors of the optimal are bolded. We see that SAM improves performance across \emph{all} model sizes.}
    \label{tab:finetune_glue}
\end{table*}

\begin{table*}[t]
    \centering
    \begin{tabular}{l|cc}
    \toprule
    Model &	Natural Q. & Web Q. \\
        \midrule
Small & 19.1 / 15.0 & 23.1 / 17.2 \\
Small + SAM (0.05) & 20.3 / 16.2 & 25.2 / 19.0 \\
\midrule
Base & 26.3 / 21.7 & 30.0 / 23.9 \\
Base + SAM (0.15) & 27.7 / 22.5 & 32.5 / 25.9 \\
\midrule
Large & 29.5 / 24.2 & 35.2 / 28.7 \\
Large + SAM (0.15) & 30.6 / 25.2 & 36.1 / 29.4 \\
\midrule
XL & 33.8 / 28.0 & 39.2 / 32.2 \\
XL + SAM (0.15) & 35.1 / 29.1 & 40.7 / 33.4 \\
\bottomrule
    \end{tabular}
    \caption{QA, 95\%.}
\end{table*}

\begin{table*}[t]
\small
    \centering
    \begin{tabular}{l|cccccc}
    \toprule
        Model &	XNLI & PAWS-X &	WikiAnn NER & XQuAD & MLQA & TyDiQA-GoldP \\
    \midrule
Small & x & x & x & x & x & x \\ 
Small + SAM (0.05) & x & x & x & x & x & x \\ 
\midrule
Base & x & x & x & x & x & 44.2 / 30.9 \\ 
Base + SAM (0.15) & x & x & x & x & x & x \\ 
\midrule
Large & x & x & x & x & x & x \\ 
Large + SAM (0.15) & x & x & x & x & x & x \\ 
\midrule
XL & x & x & x & x & x & x \\ 
XL + SAM (0.15) & x & x & x & x & x & x \\ 
        \bottomrule
    \end{tabular}
    \caption{Results for cross-lingual zero-shot transfer tasks from the multilingual T5 paper. Public checkpoints of mT5.1.1 of various sizes, which were pre-trained on the mC4 corpus, are fine-tuned on \emph{English} only data, and evaluated on test data from multiple languages. The checkpoints are fine-tuned with and without SAM for 250k steps. We see that SAM \emph{substantially} improves performance across \emph{all} model sizes.}
    \label{tab:zeroshot_mt5}
\end{table*}

\begin{table*}[t]
\small
    \centering
    \begin{tabular}{l|c|ccccccccc}
    \toprule
        Model &	SGlue &	BoolQ &	CB & 	CoPA & MultiRC &	ReCoRD &	RTE & 	WiC &	WSC \\ 
        \midrule
Small & 48.3 & 57.5 & 37.0 / 55.4 & 49.0 & 59.8 / 10.3 & 33.9 / 32.5 & 50.9 & 48.9 & 65.4 \\
Small + SAM (0.05) & 49.6 & 59.6 & 43.6 / 66.1 & 46.0 & 58.3 / 9.4 & 33.3 / 30.9 & 50.2 & 54.1 & 66.3 \\
\midrule
Base & 49.9 & 58.7 & 24.6 / 50.0 & 51.0 & 57.4 / 10.8 & 40.2 / 37.0 & 57.8 & 57.1 & 64.4 \\
Base + SAM (0.15) & 53.1 & 60.5 & 38.7 / 60.7 & 52.0 & 60.3 / 15.4 & 44.3 / 41.3 & 61.0 & 55.2 & 65.4 \\
\midrule
Large & 57.7 & 63.5 & 36.8 / 57.1 & 48.0 & 69.3 / 21.4 & 71.1 / 66.9 & 66.4 & 53.8 & 68.3 \\
Large + SAM (0.15) & 59.7 & 75.0 & 46.4 / 67.9 & 59.0 & 67.1 / 16.7 & 63.1 / 58.5 & 61.4 & 58.0 & 64.4 \\
\midrule
XL & 72.9 & 83.8 & 53.3 / 76.8 & 82.0 & 80.5 / 44.0 & 79.0 / 75.7 & 75.1 & 65.2 & 72.1 \\
XL + SAM (0.15) & 73.2 & 81.1 & 57.2 / 82.1 & 64.0 & 79.5 / 43.0 & 85.6 / 84.2 & 79.1 & 61.6 & 83.7 \\
        \bottomrule
    \end{tabular}
    \caption{SuperGLUE 100\% data where the single checkpoint that optimizes the overall score is chosen.}
\end{table*}

\begin{table*}[t]
\small
    \centering
    \begin{tabular}{l|c|ccccccccc}
    \toprule
        Model &	SGlue &	BoolQ &	CB & 	CoPA & MultiRC &	ReCoRD &	RTE & 	WiC &	WSC \\ 
        \midrule

        \bottomrule
    \end{tabular}
    \caption{SuperGLUE 5\% data where the single checkpoint that optimizes the overall score is chosen.}
\end{table*}

\begin{table*}[t]
    \centering
    \begin{tabular}{l|cc}
    \toprule
    Model &	Natural Q. & Web Q. \\
        \midrule
Small & 4.9 / 2.9 & 4.8 / 1.8 & 3.0 / 1.3 \\
Small + SAM (0.05) & 6.0 / 3.7 & 7.1 / 2.2 & 3.3 / 1.6 \\
\midrule
Base & 7.9 / 4.8 & 13.7 / 4.6 & 7.6 / 4.2 \\
Base + SAM (0.15) & 8.6 / 5.6 & 12.2 / 5.7 & 7.7 / 4.4 \\
\midrule
Large & 8.7 / 5.2 & 14.0 / 7.0 & 9.8 / 6.0 \\
Large + SAM (0.15) & 10.5 / 6.6 & 14.9 / 7.7 & 10.6 / 7.1 \\
\midrule
XL & 13.1 / 8.0 & 20.6 / 11.9 & 19.6 / 15.3 \\
XL + SAM (0.15) & 13.4 / 8.1 & 22.9 / 13.6 & 19.1 / 14.5 \\
\bottomrule
    \end{tabular}
    \caption{5\% CBQA, using 20k steps, eval every 200 steps.}
\end{table*}

\begin{table*}[t]
    \centering
    \begin{tabular}{l|cc}
    \toprule
    Model &	Natural Q. & Web Q. \\
        \midrule
Small & 4.9 / 2.9 & 4.8 / 1.8 & 3.0 / 1.3 \\
Small + SAM (0.05) & 6.0 / 3.7 & 7.1 / 2.2 & 3.3 / 1.6 \\
\midrule
Base & 7.9 / 4.8 & 13.7 / 4.6 & 7.6 / 4.2 \\
Base + SAM (0.15) & 8.6 / 5.6 & 12.2 / 5.7 & 7.7 / 4.4 \\
\midrule
Large & 8.7 / 5.2 & 14.0 / 7.0 & 9.8 / 6.0 \\
Large + SAM (0.15) & 10.5 / 6.6 & 14.9 / 7.7 & 10.6 / 7.1 \\
\midrule
XL & 13.1 / 8.0 & 20.6 / 11.9 & 19.6 / 15.3 \\
XL + SAM (0.15) & 13.4 / 8.1 & 22.9 / 13.6 & 19.1 / 14.5 \\
\bottomrule
    \end{tabular}
    \caption{100\% CBQA, using 20k steps, eval every 200 steps.}
\end{table*}

\begin{table*}[t]
    \centering
    \begin{tabular}{l|cc}
    \toprule
    Model &	Natural Q. & Web Q. \\
        \midrule
Small & 19.7 / 15.6 & 23.8 / 17.4 \\
Small + SAM (0.05) & 20.7 / 16.8 & 25.7 / 19.2 \\
\midrule
Base & 26.3 / 21.8 & 30.3 / 24.2 \\
Base + SAM (0.15) & 27.9 / 22.9 & 33.0 / 26.2 \\
\midrule
Large & 29.5 / 24.3 & 35.4 / 28.9 \\
Large + SAM (0.15) & 30.7 / 25.2 & 36.3 / 29.7 \\
\midrule
XL & 34.0 / 28.3 & 39.7 / 32.6 \\
XL + SAM (0.15) & 35.2 / 29.3 & 40.8 / 33.7 \\
\bottomrule
    \end{tabular}
    \caption{Experimental results on the Closed-Book Question Answering benchmark (dev scores for Natural Questions, Web Questions, and TriviaQA), SQUAD, and TyDiQA-GoldP. Public checkpoints of T5 (or multilingual T5 for TyDiQA) of various sizes are fine-tuned with and without SAM for 250k steps. Results are averaged over four runs, and entries that are within two standard errors of the optimal are bolded. We see that SAM improves performance across \emph{all} model sizes.}
\end{table*}

\begin{table*}[t]
    \centering
    \begin{tabular}{l|c|ccccccccc}
    \toprule
        Model &	SGlue &	BoolQ &	CB & 	CoPA & MultiRC &	ReCoRD &	RTE & 	WiC &	WSC \\ 
        \midrule
Small & 65.5 & 72.2 & 73.6 / 80.4 & 61.0 & 67.4 / 20.0 & 57.6 / 56.6 & 69.3 & 69.0 & 75.0 \\
Small + SAM (0.05) & 64.6 & 71.7 & 81.6 / 83.9 & 60.0 & 67.0 / 19.8 & 58.1 / 57.1 & 65.3 & 67.7 & 68.3 \\
\midrule
Base & 72.6 & 76.2 & 89.2 / 92.9 & 72.0 & 71.1 / 27.3 & 70.4 / 69.5 & 76.2 & 71.2 & 75.0 \\
Base + SAM (0.15) & 72.2 & 76.3 & 87.6 / 85.7 & 70.0 & 71.3 / 27.5 & 72.0 / 71.0 & 72.9 & 72.1 & 78.8 \\
\midrule
Large & 79.7 & 80.5 & 89.0 / 94.6 & 83.0 & 76.3 / 36.6 & 80.1 / 79.2 & 84.8 & 73.5 & 87.5 \\
Large + SAM (0.15) & 76.0 & 78.6 & 85.1 / 91.1 & 75.0 & 73.7 / 32.6 & 77.2 / 76.3 & 82.3 & 70.2 & 83.7 \\
\midrule
T5.1.1 XL & x & x & x & x & x & x & x & x & x \\ 
T5.1.1 XL + SAM & x & x & x & x & x & x & x & x & x \\ 
        \bottomrule
    \end{tabular}
    \caption{Experimental results (dev scores) on the SuperGLUE benchmark. Models are pre-trained with and without SAM on the C4 corpus for $500k$ and subsequently fine-tuned without SAM for $250k$ steps. NOT LOOKING GOOD.}
    \label{tab:pretrain_superglue}
\end{table*}

\begin{table*}[t]
    \centering
    \begin{tabular}{l|ccc}
    \toprule
    Model &	Natural Q. & Web Q. & TriviaQA \\
        \midrule
Small & 19.7 / 15.5 & 25.0 / 19.6 & 12.9 / 9.9 \\
Small + SAM (0.05) & 21.5 / 17.2 & 25.2 / 18.9 & 14.0 / 10.7 \\
\midrule
Base & 26.7 / 21.7 & 31.9 / 25.8 & 21.5 / 17.5 \\
Base + SAM (0.15) & 27.8 / 22.6 & 32.3 / 26.1 & 23.5 / 19.3 \\
\midrule
Large & 30.3 / 25.0 & 36.4 / 29.8 & 28.2 / 23.6 \\
Large + SAM (0.15) & 31.2 / 25.9 & 36.9 / 30.8 & 29.5 / 24.9 \\
\midrule
XL & 33.2 / 27.4 & 39.5 / 32.1 & 36.1 / 31.0 \\
XL + SAM (0.15) & 34.7 / 28.8 & 40.5 / 33.3 & 37.4 / 31.9 \\
\bottomrule
    \end{tabular}
    \caption{Experimental results (test scores) on the (full) CBQA tasks. Public checkpoints of various sizes are fine-tuned with and without SAM on the mixture of tasks for 50k steps. We see that SAM improves performance across \emph{all} model sizes.}
    \label{tab:finetune_cbqa}
\end{table*}

\begin{table*}[t]
    \centering
    \begin{tabular}{l|ccc}
    \toprule
    Model &	Natural Q. & Web Q. & TriviaQA \\
        \midrule
Small & 5.1 / 2.9 & 4.9 / 1.8 & 2.9 / 1.3 \\
Small + SAM (0.05) & 5.7 / 3.5 & 7.0 / 2.5 & 3.4 / 1.6 \\
\midrule
Base & 7.7 / 4.6 & 10.6 / 4.9 & 7.4 / 4.0 \\
Base + SAM (0.15) & 9.0 / 5.9 & 11.9 / 5.4 & 7.1 / 4.1 \\
\midrule
Large & 9.2 / 5.7 & 14.3 / 7.5 & 9.4 / 5.9 \\
Large + SAM (0.15) & 10.1 / 6.5 & 15.6 / 8.2 & 9.7 / 6.3 \\
\midrule
XL & 12.4 / 8.0 & 18.3 / 9.8 & 16.3 / 12.4 \\
XL + SAM (0.15) & 12.1 / 7.6 & 19.7 / 11.6 & 17.5 / 13.0 \\
\bottomrule
    \end{tabular}
    \caption{CBQA results when only 5\% of the training data is available.}
\end{table*}
